# Supplementary material for: Can LLMs Time Travel? Enhancing Temporal Consistency in Legal Agentic Search through Reinforcement Learning
Source: arXiv:2605.25920 source file (2026-09-19)
Supplement: Supplementary file 1 [file appendix.tex]

\newpage
\appendix
\section{Dataset}
